# Supplementary material for: An optical flow approach to tracking ship track behavior using GOES-R satellite imagery
Source: arXiv:2108.05882 source file (2023-08-14)
Supplement: Supplementary file 1 [file appendix.tex]

\section{Supplementary HYSPLIT Figures}
\setcounter{figure}{0}    

\begin{figure}[h]
		\centering
		\begin{subfigure}[t]{5.0in}
			\centering
			\includegraphics[width=\linewidth]{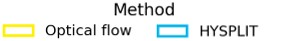}
		\end{subfigure}
		\\
		\begin{subfigure}[t]{2.75in}
			\centering
			\includegraphics[trim = 0cm 0cm 0cm 0cm, clip, width=\linewidth]{figures/2019-06-17_050238_of-hysplit.png}
			\vspace{-6mm}
			\caption{Initialization: 0 hr}
		\end{subfigure}%
		\begin{subfigure}[t]{2.75in}
			\centering
			\includegraphics[trim = 0cm 0cm 0cm 0cm, clip, width=\linewidth]{figures/2019-06-17_110238_of-hysplit.png}
			\vspace{-6mm}
			\caption{6 hr}
		\end{subfigure}
		\\
		\begin{subfigure}[t]{2.75in}
			\centering
			\includegraphics[trim = 0cm 0cm 0cm 0cm, clip, width=\linewidth]{figures/2019-06-17_170238_of-hysplit.png}
			\vspace{-6mm}
			\caption{12 hr}
		\end{subfigure}%
		\begin{subfigure}[t]{2.75in}
			\centering
			\includegraphics[trim = 0cm 0cm 0cm 0cm, clip, width=\linewidth]{figures/2019-06-17_230238_of-hysplit.png}
			\vspace{-6mm}
			\caption{18 hr}
		\end{subfigure}
	
	\caption{Shown are the combined results of HYSPLIT trajectory analysis and optical flow approach for the June case study.  Both HYSPLIT and optical flow were initialized on June 17, 2019, at 05:02 UTC, shown in (a), and snapshots are shown (b) 6, (c) 12, and (d) 18 hr later.  The HYSPLIT analyses were initialized at four different altitudes for comparison. Though both methods agree with the motion of the ship tracks, some of the HYSPLIT projections appear to accumulate error over time.  The ship tracks remain clearly visible 18 hr after initialization}
	\label{fig:lk-hysplit_june_supp}
\end{figure}

\begin{figure}[h]
		\centering
		\begin{subfigure}[t]{5.0in}
			\centering
			\includegraphics[width=\linewidth]{figures/legend_reformat.jpg}
		\end{subfigure}
		\\
		\begin{subfigure}[t]{2.75in}
			\centering
			\includegraphics[trim = 0cm 0cm 0cm 0cm, clip, width=\linewidth]{figures/2019-02-20_170238_of-hysplit.png}
			\vspace{-6mm}
			\caption{Initialization: 0 hr}
		\end{subfigure}%
		\begin{subfigure}[t]{2.75in}
			\centering
			\includegraphics[trim = 0cm 0cm 0cm 0cm, clip, width=\linewidth]{figures/2019-02-20_210238_of-hysplit.png}
			\vspace{-6mm}
			\caption{4 hr}
		\end{subfigure}
		\\
		\begin{subfigure}[t]{2.75in}
			\centering
			\includegraphics[trim = 0cm 0cm 0cm 0cm, clip, width=\linewidth]{figures/2019-02-21_010238_of-hysplit.png}
			\vspace{-6mm}
			\caption{8 hr}
		\end{subfigure}%
		\begin{subfigure}[t]{2.75in}
			\centering
			\includegraphics[trim = 0cm 0cm 0cm 0cm, clip, width=\linewidth]{figures/2019-02-21_050238_of-hysplit.png}
			\vspace{-6mm}
			\caption{12 hr}
		\end{subfigure}
	
	\caption{Shown are the combined results of HYSPLIT trajectory analysis and optical flow approach for the February case study.  Both methods were initialized on February 20, 2019, at 17:02 UTC, shown in (a), and snapshots are shown (b) 4, (c) 8, and (d) 12 hr later.  The HYSPLIT analyses were initialized at four different altitudes for comparison.  Though both methods agree with the motion of the ship tracks, some of the HYSPLIT projections appear to accumulate error over time.  The ship tracks remain visible 8 hr after initialization}
	\label{fig:lk-hysplit_feb_supp}
\end{figure}

\begin{figure}[h]
		\centering
		\begin{subfigure}[t]{5.0in}
			\centering
			\includegraphics[width=\linewidth]{figures/legend_reformat.jpg}
		\end{subfigure}
		\\
		\begin{subfigure}[t]{2.75in}
			\centering
			\includegraphics[trim = 0cm 0cm 0cm 0cm, clip, width=\linewidth]{figures/2019-04-23_190238_of-hysplit.png}
			\vspace{-6mm}
			\caption{Initialization: 0 hr}
		\end{subfigure}%
		\begin{subfigure}[t]{2.75in}
			\centering
			\includegraphics[trim = 0cm 0cm 0cm 0cm, clip, width=\linewidth]{figures/2019-04-24_000238_of-hysplit.png}
			\vspace{-6mm}
			\caption{5 hr}
		\end{subfigure}
		\\
		\begin{subfigure}[t]{2.75in}
			\centering
			\includegraphics[trim = 0cm 0cm 0cm 0cm, clip, width=\linewidth]{figures/2019-04-24_040238_of-hysplit.png}
			\vspace{-6mm}
			\caption{9 hr}
		\end{subfigure}%
		\begin{subfigure}[t]{2.75in}
			\centering
			\includegraphics[trim = 0cm 0cm 0cm 0cm, clip, width=\linewidth]{figures/2019-04-24_080238_of-hysplit.png}
			\vspace{-6mm}
			\caption{13 hr}
		\end{subfigure}

	\caption{Shown are the combined results of HYSPLIT trajectory analysis and optical flow approach for the April case study.  Both methods were initialized on April 24, 2019, at 19:02 UTC, shown in (a).  GOES-R ABI data from 22:58 to midnight on April 24, 2019, is unavailable, so snapshots are shown (b) 5, (c) 9, and (d) 13 hr later.  The HYSPLIT predictions were initialized at four different altitudes for comparison.  The ship tracks remain clearly visible 9 hr after initialization}
	\label{fig:lk-hysplit_apr_supp}
\end{figure}

\clearpage
\section{Details on sunset/sunrise transitions using solar zenith angle}\label{sec:supp_sza}

We determined the starting and ending frames of a diurnal transition using calculated solar zenith angles at the right and left perimeter of our tracking box, respectively. 
These angles were calculated using the National Renewable Energy Laboratory’s Solar Position Algorithm \citep{nrel2008}, which calculates the sun's apparent altitude with a precision of about 0.0003 degrees given the date, time, and location. 
For a given frame, the minimum and maximum angles are used for both the right and left edges of the tracking box to determine the beginning and end of a diurnal transition.
Thresholds for the start and end of each transition were chosen empirically and conservatively to ensure the transition periods are estimated accurately.

Specifically, let $\alpha_r$ and $\alpha_l$ be vectors of pixel solar zenith angles for the right and left half of the tracking box perimeter, respectively, and let $c, d \in \mathbb{R}$ such that $0< c < d$ be the thresholds for transition periods. Then a diurnal transition is occurring if the following condition is true:

\begin{equation*}
(\hbox{min}(\alpha_r) < d \cap \hbox{max}(\alpha_l) > c ) \cup (\hbox{max}(\alpha_r) > c \cap \hbox{min}(\alpha_l) < d ).
\end{equation*}

The first set in the union describes a sunrise and the second describes a sunset.
A demonstration of this condition is displayed in figure \ref{fig:transitions} , which shows the diurnal pattern of rising and falling slopes of $\hbox{max}(\alpha_l)$, $\hbox{min}(\alpha_r)$, $\hbox{max}(\alpha_r)$, and $\hbox{min}(\alpha_l)$ for the February case study. 
The sunrise boundary begins at the frame in which $\hbox{min}(\alpha_r) < d$ on a falling slope of $\hbox{min}(\alpha_r)$ values and ends at the frame where $\hbox{max}(\alpha_l) \leq c.$
The sunset boundary begins at the frame in which $\hbox{max}(\alpha_r) > c$ on a rising slope of $\hbox{max}(\alpha_r)$ values and ends at the frame where $\hbox{min}(\alpha_l) \geq d$.

To determine empirical values for $c$ and $d$, we sampled a total of eight sunrise and nine sunset images from multiple dates. Using ten points manually selected from each image where sunrise or sunset significantly impacted cloud radiance, we derived a total of 160 solar zenith angles. Figures \ref{fig:transition_points} (a) and (b) show an example of selected points along the start of a sunrise and sunset transition, respectively.

%\begin{equation*}
%( min(\alpha_r) < d \cap max(\alpha_l) > c ) \cup ( max(\alpha_r) > c \cap min(\alpha_l) < d ).
%\end{equation*}

%Figures \ls{sza figs for sunrise and sunset} demonstrates where sunrise and sunset transitions occur over a 24 hour period. Sunrise is expected on the increasing slope between midnight and high noon, while sunset is expected on the decreasing slope between high noon and midnight\ls{this is incorrect but simply a place holder for a similar statement}.
%The sunrise boundary begins at the frame in which $min(\alpha_r) < d)$ on a falling slope of $min(\alpha_r)$ values and the sunset boundary begins at the frame in which $max(\alpha_r) > c)$ on a rising slope of $max(\alpha_r)$ values. Figures \ls{insert figures} demonstrates the diurnal pattern and rising and falling slopes of  $min(\alpha_r)$ and $max(\alpha_r).$
%We initially chose a sunrise threshold of $d=91^\circ$ or the $95^{th}$ percentile of sampled angles indicating sunrise. Although in application, we found a good estimate of the start of sunrise to be when the minimum angle at the right hand side of the box falls below 96$^\circ$. Similarly, we found that the maximum angle on the right side of the box exceeds $84^\circ$ is a good indicator of the start of a sunset transition.  
\begin{figure}[h]
		\centering
		\begin{subfigure}[t]{2.75in}
			\centering
			\includegraphics[trim = 0cm 0cm 0cm 0cm, clip, width=\linewidth]{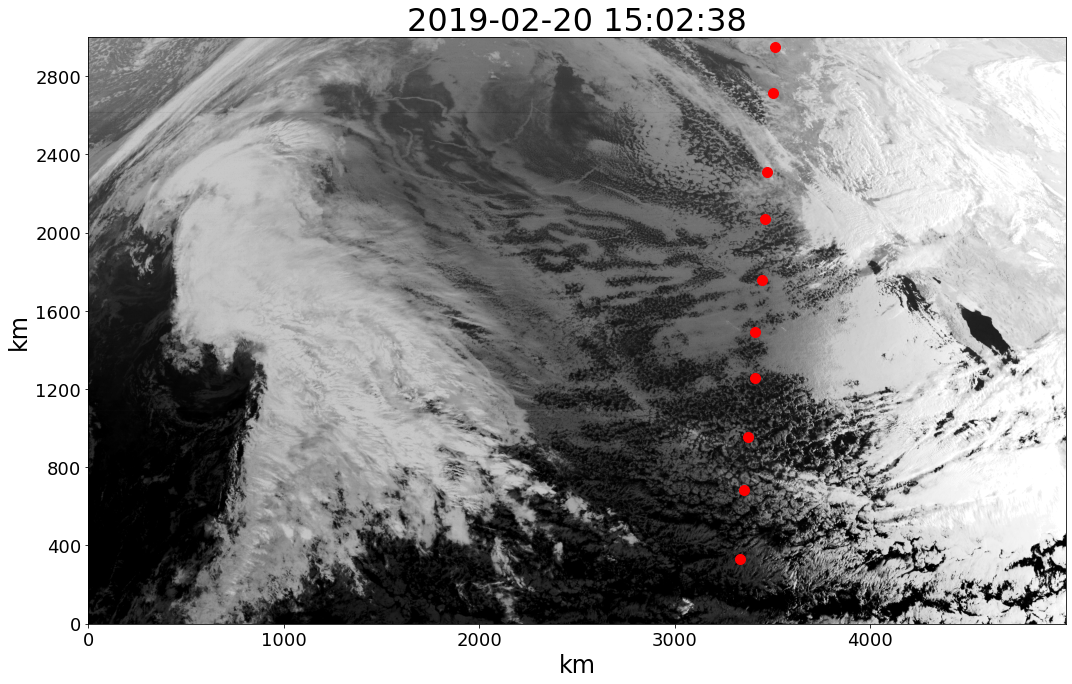}
			%\vspace{-6mm}
			\caption{Sunrise}
		\end{subfigure}%
		\begin{subfigure}[t]{2.75in}
			\centering
			\includegraphics[trim = 0cm 0cm 0cm 0cm, clip, width=\linewidth]{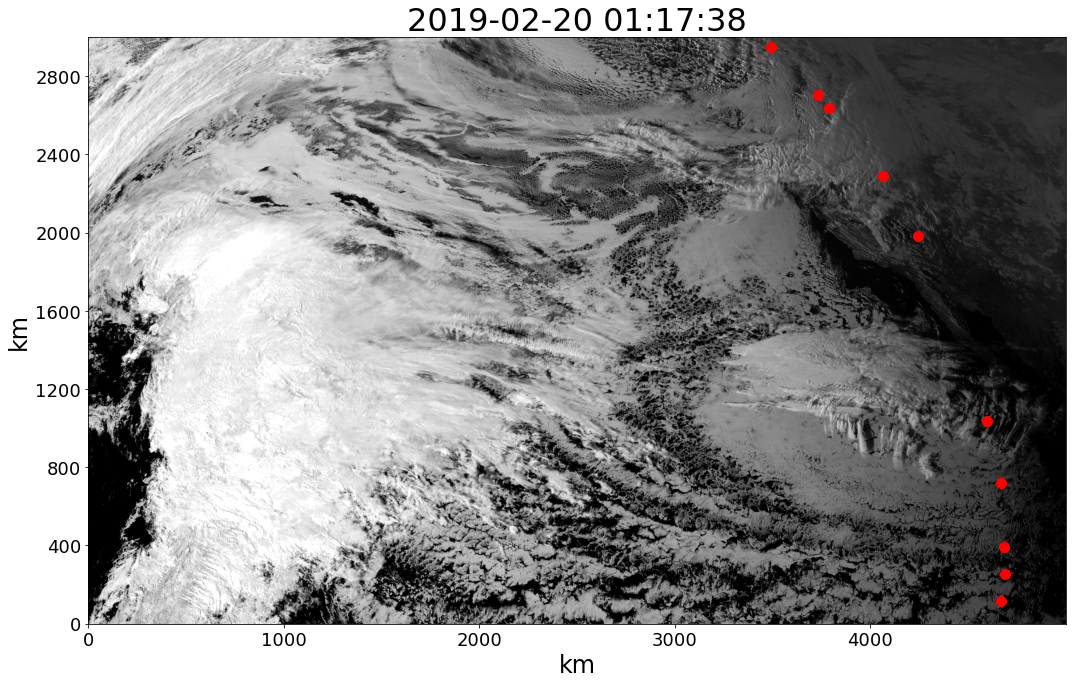}
			%\vspace{-6mm}
			\caption{Sunset}
		\end{subfigure}
	
	\caption{Examples of selected observations (red points) for a sunrise (a) and sunset (b) transition on February $20^{th}$}
	\label{fig:transition_points}
\end{figure}

%The ending frame of sunrise and sunset transitions are identified using angle computations on the left side of the box. The sunrise boundary then ends at the frame in which $max(\alpha_l) \leq c$; the sunset boundary ends at the frame where $min(\alpha_l) \geq d$. Then a sunrise or sunset transition is occurring if the following condition is true:

%\begin{equation*}
%( min(\alpha_r) < d \cap max(\alpha_l) > c ) \cup ( max(\alpha_r) > c \cap min(\alpha_l) < d ).
%\end{equation*}

We initially chose a sunrise threshold of $d=91^\circ$ or the $95^{th}$ percentile of sampled angles during a sunrise event. Although in application, we found a better estimate of the start of sunrise to be when the minimum angle at the right hand side of the box falls below 96$^\circ$. Similarly, we found that when the maximum angle on the right side of the box exceeds $84^\circ$, it is a good indicator of the start of a sunset transition.  The last frame of a sunrise transition was determined when the maximum angle falls below $84^\circ$ and sunset transitions completed when the minimum angle is above $96^\circ.$ Using the solar zenith angle, we found diurnal transitions to be reliably predictable. 

\begin{figure}[h]
	\centering
	\includegraphics[trim = 0cm 0cm 0cm 0cm, clip, width=0.8\linewidth]{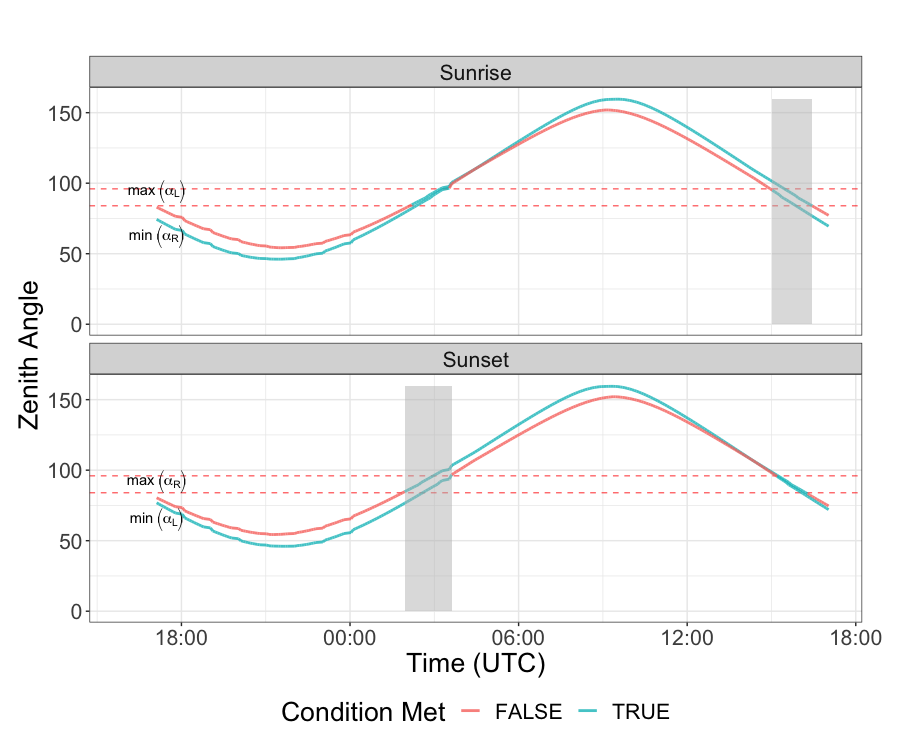}
	\caption{This figure demonstrates the diurnal cycle of the minimum and maximum solar zenith angles for the right and left side of the tracking box over a 25 hour period starting on February $20^{th}$ at 17:00 UTC and ending on February $21^{th}$ at 18:00 UTC. The top figure shows the behavior of $\hbox{max}(\alpha_L)$ $\hbox{min}(\alpha_R)$, which indicate the start and stop of a sunrise transition while the bottom figure shows the behavior of $\hbox{max}(\alpha_R)$ $\hbox{min}(\alpha_L)$, which indicate the start and stop of a sunset transition. The vertical grey boxes indicate the time period where the transition conditions are met and thus the time periods for a sunrise or sunset event}
	\label{fig:transitions}
\end{figure}
